# Supplementary material for: Geo6D: Geometric Constraints Learning for 6D Pose Estimation
Source: arXiv:2210.10959 source file (2023-08-22)
Supplement: Supplementary file 1 [file appendix.tex]

\definecolor{codeblue}{rgb}{0.25,0.5,0.5}
\definecolor{keyword}{rgb}{0.8, 0.25, 0.5}
\newcommand{\listingsttfamily}{\fontfamily{pcr}\small}
\lstset{
        backgroundcolor=\color{white},
        basicstyle=\fontsize{8pt}{8pt}\listingsttfamily,
        columns=fullflexible,
        breaklines=False,
        commentstyle=\fontsize{8pt}{8pt}\color{codeblue},
        keywordstyle=\fontsize{8pt}{8pt}\color{keyword},
}
In this supplemental material, we demonstrate the pseudo-code of our 5D anchor mechanism, implementation details of experiments, and quantitative and qualitative results on the YCB-Video Dataset. Following that, there is an analysis of translation distribution and limitations of 5D anchor.
\section{Algorithm Pseudocode}
We provide the pseudocode of our 5D anchor generation and anchor-based projection as Algorithm~\ref{alg:pseudocode}.
\begin{figure}[htp]
	\centering
	%\resizebox{\linewidth}{!}{
		\begin{minipage}{\linewidth}
			\begin{algorithm}[H]
				\caption{5D anchor mechanism in a PyTorch-like style.}
				\label{alg:pseudocode}
				\begin{algorithmic}
				    \STATE \textbf{Input}: $U, V, D, T, K, mask, bbox$
				    \STATE \textbf{Output}: $\Delta U, \Delta V, \Delta X, \Delta Y, \Delta D, \Delta T$
				\end{algorithmic}
				\begin{lstlisting}[language=python,tabsize=4,showtabs]
# U,V: predefined 2D coordinates on the 
# image plane (H, W)
# D: depth image (H, W)
# T: 3 Degree of freedom for 
# Translation  (3,)
# K: camera intrinsic matrix (3, 3)
# mask: segmentation result from the
# first stage. (H, W)
# bbox: predicted object bounding box
# from the first stage. (4,)

# core value from camera intrinsic matrix
f_x, c_x = K[0, 0], K[0, 2]
f_y, c_y = K[1, 1], K[1, 2]

# depth image project to 3D point
u_i = U
v_i = V
d_i = D
x_i = (u_i - c_x) / f_x * d_i
y_i = (v_i - c_y) / f_y * d_i

# 5D anchor generation
# RoI center x,y,width,and height
c_col, c_row, w, h = bbox 
u_0 = U[c_row, c_col]
v_0 = V[c_row, c_col]
# mean foreground pixel's depth
d_0 = depth[mask].mean() 
x_0 = (u_0 - c_x) / f_x * d_0
y_0 = (v_0 - c_y) / f_y * d_0

# anchor-based projection
delta_u = u_i - u_0
delta_v = v_i - v_0
delta_x = x_i / d_i - x_0 / d_0
delta_y = y_i / d_i - y_0 / d_0
delta_d = d_i - d_0

T_x, T_y, T_d = T
delta_T = [T_x - x_0, T_y - y_0, T_d - d_0]

\end{lstlisting}
			\end{algorithm}
			%}
	\end{minipage}
\end{figure}

\begin{table*}[htb]
\begin{center}
\resizebox{0.9\linewidth}{!}{
\begin{tabular}{l|c|c|c|c|c|c|c|c|c|c|c|c|c|c}
    \toprule
 & \multicolumn{2}{c|}{PoseCNN}  & \multicolumn{2}{c|}{DenseFusion} & \multicolumn{2}{c|}{PVN3D} & \multicolumn{2}{c|}{FFB6D} & \multicolumn{2}{c|}{Uni6D} & \multicolumn{2}{c|}{Uni6Dv2} & \multicolumn{2}{c}{Uni6Dv3} \\ 
    \midrule
 Object & \small{ADD-S} & \small{ADD(S)} & \small{ADD-S} & \small{\small{ADD(S)}} & \small{ADD-S} & \small{ADD(S)} & \small{ADD-S} & \small{ADD(S)} & \small{ADD-S} &\small{ADD(S)} & \small{ADD-S} &\small{ADD(S)} & \small{ADD-S} &\small{ADD(S)}\\ \midrule
        002\_master\_chef\_can & 83.9 & 50.2 & 95.3 & 70.7 & 96 & 80.5 & 96.3 & 80.6 & 95.4 & 70.2 & 96.0 & 74.2 & 95.8 & 78.4 \\
        003\_cracker\_box & 76.9 & 53.1 & 92.5 & 86.9 & 96.1 & 94.8 & 96.3 & 94.6 & 91.8 & 85.2 & 96.0 & 94.2 & 96.0 & 94.0\\ 
        004\_sugar\_box & 84.2 & 68.4 & 95.1 & 90.8 & 97.4 & 96.3 & 97.6 & 96.6 & 96.4 & 94.5 & 97.6 & 96.6 & 97.6 & 96.5\\ 
        005\_tomato\_soup\_can & 81.0 & 66.2 & 93.8 & 8.47 & 96.2 & 88.5 & 95.6 & 89.6 & 95.8 & 85.4 & 96.1 & 86.6 & 95.9 & 87.0\\
        006\_mustard\_bottle & 90.4 & 81.0 & 95.8 & 90.9 & 97.5 & 96.2 & 97.8 & 97.0 & 95.4 & 91.7 & 97.8 & 96.7 & 98.0 & 96.6\\   % drop
        007\_tuna\_fish\_can & 88.0 & 70.7 & 95.7 & 79.6 & 96.0 & 89.3 & 96.8 & 88.9 & 95.2 & 79.0 & 96.3 & 76.0 & 96.0 & 74.1\\ 
        008\_pudding\_box & 79.1 & 62.7 & 94.3 & 89.3 & 97.1 & 95.7 & 97.1 & 94.6 & 94.1 & 89.8 & 96.6 & 94.7 & 97.4 & 96.0\\ 
        009\_gelatin\_box & 87.2 & 75.2 & 97.2 & 95.8 & 97.7 & 96.1 & 98.1 & 96.9 & 97.4 & 96.2 & 98.0 & 97.0 & 97.9 & 97.1\\  % drop
        010\_potted\_meat\_can & 78.5 & 59.5 & 89.3 & 79.6 & 93.3 & 88.6 & 94.7 & 88.1 & 93.0 & 89.6 & 95.7 & 91.9 & 95.9 & 92.5\\ 
        011\_banana & 86.0 & 72.3 & 90.0 & 76.7 & 96.6 & 93.7 & 97.2 & 94.9 & 96.4 & 93.0 & 98.0 & 96.9 & 97.7 & 95.9\\ % drop
        019\_pitcher\_base & 77.0 & 53.3 & 93.6 & 87.1 & 97.4 & 96.5 & 97.6 & 96.9 & 96.2 & 94.2 & 97.5 & 96.9 & 97.4 & 96.7\\  % drop
        021\_bleach\_cleanser & 71.6 & 50.3 & 94.4 & 87.5 & 96.0 & 93.2 & 96.8 & 94.8 & 95.2 & 91.1 & 97.0 & 95.3 & 97.0 & 95.4\\  % drop
        \textbf{024\_bowl} & 69.6 & 69.6 & 86.0 & 86.0 & 90.2 & 90.2 & 96.3 & 96.3 & 95.5 & 95.5 & 96.8 & 96.8 & 95.7 & 95.7\\ 
        025\_mug & 78.2 & 58.5 & 95.3 & 83.8 & 97.6 & 95.4 & 97.3 & 94.2 & 96.6 & 93.0 & 97.7 & 96.3 & 97.3 & 94.7\\  % drop
        035\_power\_drill & 72.7 & 55.3 & 92.1 & 83.7 & 96.7 & 95.1 & 97.2 & 95.9 & 94.7 & 91.1 & 97.6 & 96.8 & 97.4 & 96.4\\  % drop
        \textbf{036\_wood\_block} & 64.3 & 64.3 & 89.5 & 89.5 & 90.4 & 90.4 & 92.6 & 92.6 & 94.3 & 94.3 & 96.1 & 96.1 & 95.7 & 95.7\\ 
        037\_scissors & 56.9 & 35.8 & 90.1 & 77.4 & 96.7 & 92.7 & 97.7 & 95.7 & 87.6 & 79.6 & 95.0 & 90.3 & 94.2 & 88.4\\  % drop
        040\_large\_marker & 71.7 & 58.3 & 95.1 & 89.1 & 96.7 & 91.8 & 96.6 & 89.1 & 96.7 & 92.8 & 97.0 & 93.1 & 97.6 & 94.4\\
        \textbf{051\_large\_clamp} & 50.2 & 50.2 & 71.5 & 71.5 & 93.6 & 93.6 & 96.8 & 96.8 & 95.9 & 95.9 & 97.0 & 97.0 & 96.4 & 96.4\\  % drop
        \textbf{052\_extra\_large\_clamp} & 44.1 & 44.1 & 70.2 & 70.2 & 88.4 & 88.4 & 96.0 & 96.0 & 95.8 & 95.8 & 96.5 & 96.5 & 95.9 & 95.9\\  % drop
        \textbf{061\_foam\_brick} & 88.0 & 88.0 & 92.2 & 92.2 & 96.8 & 96.8 & 97.3 & 97.3 & 96.1 & 96.1 & 97.4 & 97.4 & 96.01 & 96.01\\ % drop \midrule[1pt]
        \midrule
        Avg & 75.8 & 59.9 & 91.2 & 82.9 & 95.5 & 91.8 & 96.6 & 92.7 & 95.2 & 88.8 & 96.8 & 91.5 & 96.6 & 91.5\\   \bottomrule
\end{tabular}}
\end{center}     
\caption{Evaluation results on the YCB-Video dataset. Symmetric objects are denoted in bold.}
\label{tab:ycb}
\end{table*}

\section{Implementation Details}

\subsection{Details of Uni6Dv3}
We provide the details about the pose estimation network of Uni6Dv3 in this section. The settings of instance segmentation network and initialization of first convolutional layer are same with Uni6Dv2~\cite{uni6dv2}, and we change the $(U,V,X,Y,D)$ value of input as $(\Delta U,\Delta V,\Delta X,\Delta Y,\Delta D)$.

\textbf{For Occlusion LineMOD and LineMOD}:
\begin{itemize}
%    \item Input data: $\rgb,\Delta U,\Delta V,\Delta X,\Delta Y,\Delta D,\nrm$
    \item Data augmentation: 
    \begin{enumerate}
        \item Multi-scale training: short edge random from [320, 400, 480, 540, 600],and the max size of long edge is 800.
        \item Random crop: 0.3 probability, and keep all objects.
        \item Random erase (Occlusion LineMOD): 1.0 probability, erasing ratio random from 0.2 to 1.0.
    \end{enumerate}
    \item Training:
    \begin{enumerate}
        \item Pretrained weight: ImageNet(ResNet50).
        \item Schedule: 40 epochs, MultiStepLR with [15, 25, 35] schedule and 0.1$\times$decay.
        \item Optimizer: SGD, momentum is 0.9, weight\_deacy is 0.0001, warm-up 4 epochs.
    \end{enumerate}
    \item Loss function:
    \begin{enumerate}
        \item Loss function: $\mathcal{L} = \lambda_0 \cdot \mathcal{L}_{pose} + \mathcal{L}_{depth}$. 
        \item $\lambda_0$ is changed in training: 1-15 epoch is 1, 16-25 epoch is 5, 26-35 epoch is 10 and 36-40 epoch is 20.
    \end{enumerate}
\end{itemize}

\textbf{For YCB-Video}:
\begin{itemize}
%    \item Input data: $\rgb,\Delta U,\Delta V,\Delta X,\Delta Y,\Delta D,\nrm$
    \item Data augmentation: 
    \begin{enumerate}
        \item Multi-scale training: short edge random from [180, 200, 224, 250, 270], and the max size of long edge is 360.
        \item Random crop: 1.0 probability, expand ROI by 0.3 and keep the object.
        \item Mask dilation and erosion: 0.75 probability, the kernel size random from 3, 5 and 7.
    \end{enumerate}
    \item Training:
    \begin{enumerate}
        \item Pretrained weight: ImageNet(ResNet50).
        \item Schedule: 40 epochs, MultiStepLR with [15, 25, 35] schedule and 0.1$\times$decay.
        \item Optimizer: SGD, momentum is 0.9, weight\_deacy is 0.0001, warm-up 4 epochs.
    \end{enumerate}
    \item Loss function:
    \begin{enumerate}
        \item Loss function: $\mathcal{L} = \lambda_0 \cdot \mathcal{L}_{pose} + \mathcal{L}_{depth}$. 
        \item $\lambda_0$ is changed in training: 1-15 epoch is 1, 16-25 epoch is 5, 26-35 epoch is 10 and 36-40 epoch is 20.
    \end{enumerate}
\end{itemize}

\subsection{Details of ES6D* and ES6D* + 5D anchor}
%ES6D~\cite{mo2022es6d} densely regresses offsets from visible points to the centroid point in 3D space. However, the mismatch between the input and output limits the accuracy of pose estimation.
We employ 5D anchor on the latest direct method ES6D~\cite{es6d}, which adopts $\rgb, \Delta X, \Delta Y$ and $ \Delta D$ as input data. Different from 5D anchor following anchor-based projection, it uses $X, Y, D$ subtracts the mean value $X_c, Y_c, D_c$ and scales it to $[-1, 1]$. Since ES6D has no implementation on the Occlusion LineMOD dataset, we implement it's normalized input and dense prediction design, and select the ADD Loss for fair comparison. To apply our 5D anchor, the geometric information in input data is adjusted by inserting $\Delta U, \Delta V$ and recalculating the $\Delta X, \Delta Y, \Delta D$ based on the projection equation. Besides, the regression target of network convert to the physical offset distance for matching the anchor-based projection equation. 
Since ES6D is not intended for the Occlusion LineMOD, we modify the code and use ES6D* to denote our implementation. 
%Compared with original strategy, our 5D anchor achieve 3.5\% improvement.

\textbf{For ES6D*}:
\begin{itemize}
    % \item Input data: $\rgb, \Delta X,\Delta Y,\Delta D$.
    \item Anchor generation strategy: 
    \begin{enumerate}
        \item Input: $\Delta x=(x_i-x_c)*\gamma, \Delta y=(y_i-y_c)*\gamma, \Delta d=(d_i-d_c)*\gamma$, $\gamma$ is scale factor.
        \item Output: Scaled offsets of visible points to centroid.
    \end{enumerate}
    \item Network design:
    \begin{enumerate}
        \item Backbone: ImageNet(ResNet18) without pretrain.
        \item Regression head: Per-pixel dense regression.
        \item Optimizer: SGD, momentum is 0.9, weight\_deacy is 0.0001, warm-up 4 epochs.
    \end{enumerate}
    \item Loss function: ADD loss.
\end{itemize}

\textbf{For ES6D* + 5D anchor}:
\begin{itemize}
    % \item Input data: $\rgb,\Delta U,\Delta V,\Delta X,\Delta Y,\Delta D$.
    \item Anchor generation strategy: 
    \begin{enumerate}
        \item Input: $ \Delta u=u_i-u_0, \Delta v=v_i-v_0, \Delta x=\frac{x_i}{d_i}-\frac{x_0}{d_0}, \Delta y=\frac{y_i}{d_i}-\frac{y_0}{d_0},\Delta d=d_i-d_0$.
        \item Output: Physical offset distance to origin.
    \end{enumerate}
    \item Network design:
    \begin{enumerate}
        \item Backbone: ImageNet(ResNet18) without pretrain.
        \item Regression head:  Per-pixel dense regression.
        \item Optimizer: SGD, momentum is 0.9, weight\_deacy is 0.0001, warm-up 4 epochs.
    \end{enumerate}
    \item Loss function: ADD loss.
\end{itemize}

\subsection{Details of Dense Prediction and Sparse Prediction}
\begin{figure}[t]
    \centering
    \includegraphics[width=0.5\textwidth]{figures/dense_head.png}
    \caption{Details of dense prediction head. Features of all proposals extracted through RoI-Align are used as the input.
}
    \label{fig:dense_head}
\end{figure}

\begin{figure*}[t]
    \centering
    \includegraphics[width=0.9\textwidth]{figures/ycb_vis.png}
    \caption{Qualitative results of reducing data dependency on the YCB-Video dataset.
}
    \label{fig:ycb_vis}
\end{figure*}
We use the dense prediction head to replace the RT head in Uni6Dv2 as our dense prediction method, and the Uni6Dv3 as our sparse method. The implementation details of dense prediction head are shown in Fig~\ref{fig:dense_head}, where the stride of Conv2D and ConvTranspose2d is 1 and 2 respectively, and the feature planes is 256. 

\section{Quantitative Results on YCB-Video Dataset}
Experimental results of YCB-Video dataset are reported in Table~\ref{tab:ycb}, our approach achieves 96.6\% AUC of ADD-S and 91.5\% AUC of ADD(S), which is comparable with state-of-the-art. Because there is no translation distribution gap between training and test data, our 5D anchor have no significant advantage.
More visualization results show in the video of the supplementary material. 

\section{Qualitative results of reducing data dependency on YCB-Video Dataset}
% We use fewer training data to explore the advantage of the 5D anchor mechanism, and give more comparison results between Uni6Dv3 and Uni6Dv2 method in Fig~\ref{fig:ycb_vis}
As demonstrated in Fig~\ref{fig:ycb_vis}, we visualize the prediction results of Uni6Dv2 and Uni6D v3 under 1\% and 10\% training data on the YCB-Video dataset, which verifies that introducing the 5D anchor has better robustness in the case of reduced data volume.
\section{Translation Distribution on Occlusion LineMOD Dataset}
As shown in Table\ref{tab:distribution}, we analyse the translation distribution and take the object ``eggbox" as example. For original training and test dataset, there is a obvious distribution gap, $T_x$ range in (-0.33, 0.29) and (-0.11, 0.61) respectively. When adopting the 5D anchor, $T_x$ range in (-0.07, 0.07) and (-0.05, 0.06) in training and test data, respectively. More importantly, the variance of $X,Y, Z$ distinctly drop 100 times after employing the 5D anchor.
\begin{table}[h]
   \centering
   \resizebox{0.99\linewidth}{!}{
     \begin{tabular}{l|c|c|c|c|c|c|c}
         \toprule
       \multicolumn{2}{c|}{Setting}  & \multicolumn{3}{c|}{Variance} & \multicolumn{3}{c}{Range} \\ 
         \midrule
      \small{dataset} & \small{5D anchor} & \small{X} & \small{Y} & \small{Z}  & \small{X} & \small{Y} & \small{Z} \\ \midrule[1pt]
             Training &   & $6e^{-3}$ & $6e^{-3}$ & $3e^{-2}$ & $(-0.33, 0.29)
 $ & $(-0.27, 0.32)$ & $(0.37, 1.3)$ \\
               Training & \checkmark & $2e^{-5}$ & $2e^{-5}$ & $9e^{-5}$ & $(-0.07, 0.07)$ & $(-0.06, 0.06)$ & $(-0.04, 0.07)$ \\
               Test &  & $1e^{-2}$ & $2e^{-2}$ & $2e^{-2}$ & $(-0.11, 0.61)$ & $(-0.49, 0.3)$ & $(0.57, 1.47)$  \\ 
             Test & \checkmark & $2e^{-4}$ & $1e^{-4}$ & $1e^{-4}$ & $(-0.05, 0.06)$ &$(-0.06, 0.03)$ & $(-0.03, 0.07)$  \\ 
       \bottomrule
     \end{tabular}}
       \caption{3D translation distribution comparison}
         \label{tab:distribution}
 \end{table}
 
\section{Limitations}
%Although we significantly outperform the state-of-the-art on Occlusion LineMOD, there is still room for performance improvement. This part is mainly the scenes with heavy occlusion. How to get a stable anchor point when the occlusion is heavy is a direction worth exploring, which we leave for future works. 
In this paper, we select a simple and effective anchor generation strategy to make our 5D anchor general. For challenge scenes with insufficient visible points, the mean depth value is more likely to be disturbed by the sensor noise or background noise, limiting the stability of the anchor.
When the center of ROI is located on the outside of the object, the distance from the anchor point to the origin is relatively far.
We believe that the cluster method can alleviate it by filtering the outliers and searching the centroid.
%but the time-consuming pre-processing increases the network burden and is heavy in practice.
However, introducing extra pre-processing violates the conception of simple and effective design in Uni6D series. We will attempt to improve it in the future work.

% Moreover, the proposed 5D anchor can reduce the data demand of training, therefore may have a negative impact on object pose annotation workers.
% In this paper, we select a simple and effective anchor generation strategy to generalize our 5D anchor. For challenge scene with insufiicent visible point or ,   
